# Supplementary material for: Microscopic Phase-Field Modeling
Source: arXiv:2410.08180 ancillary file (2025-10-29)
Supplement: Supplementary file 1 [file Supplemental_Material.pdf]

# Supplemental Material: First-Principles Phase-Field Modeling

Jaehyeok Jin\* and David R. Reichman†

Department of Chemistry, Columbia University, New York, New York 10027, USA

(Dated: October 10, 2024)

## I. MICROSCOPIC-MESOSCOPIC LINK

Figure S1 summarizes the primary objective of this paper, which provides a hierarchical strategy for constructing a microscopic phase-field model. It is completely impractical to rigorously derive a phase-field dynamics model spanning a wide range of length and time scales directly from the fully atomistic level description (approximately limited to nano-meters/seconds), as this generally leads to overfitting problems when attempting to reduce millions of degrees of freedom into a small set of parameters. Here, we use coarse-graining (CG) as a means to accomplish this goal.

## II. DERIVATION OF MICROSCOPIC DESCRIPTION

### A. Microscopic Order Parameter

#### 1. Design principle of $\rho_I$

In this subsection, we outline the principles used to construct the microscopic order parameter  $\rho_I$  [Eq. (3)], which is derived from microscopic simulation trajectories to specify the bottom-up phase-field variable  $\phi_I$  [Eq. (4)].

We first determine the coefficient  $c$  in  $\rho_I = \sum_J \exp(-|\mathbf{R}_I - \mathbf{R}_J|^2/c)$ , corresponding to the variance of the Gaussian, for  $\rho_I$  by constructing the histogram of squared distances without any prefactor:

$$a_I = \sum_J |\mathbf{R}_I - \mathbf{R}_J|^2, \quad (\text{S1})$$

over the course of CG simulations from  $\tau_{\text{CG}} = 0$  to  $2 \times 10^6$  as illustrated in Fig. 1(a). Figure S2 depicts the histogram distributions of the squared distance order parameter (units in  $\text{\AA}^2$ ).

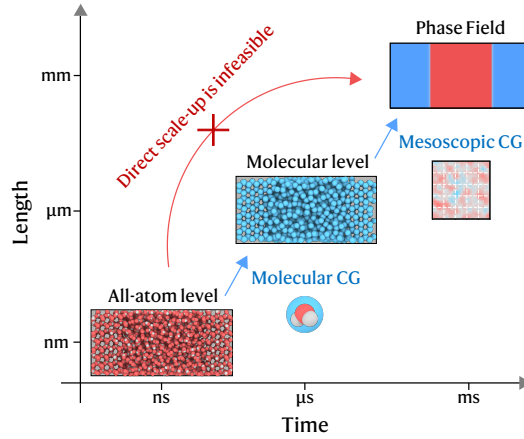

FIG. S1. Schematic diagram highlighting the concept of utilizing hierarchical coarse-graining approaches [(1) molecular coarse-graining and (2) mesoscopic coarse-graining] for constructing a phase-field representation of the water-ice interface solely derived from the fully atomistic system.

\* jj3296@columbia.edu

† drr2103@columbia.edu

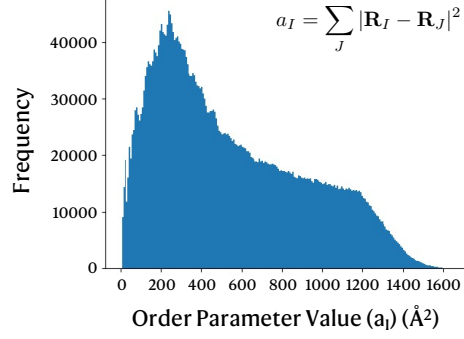

FIG. S2. Histogram distributions of the squared distance order parameter  $a_I$  during the single-site CG simulation for  $2 \times 10^6 \tau_{CG}$  as illustrated in Fig. 1(a). The median of the distribution is located near  $a_I \approx 554$  ( $\text{\AA}^2$ ).

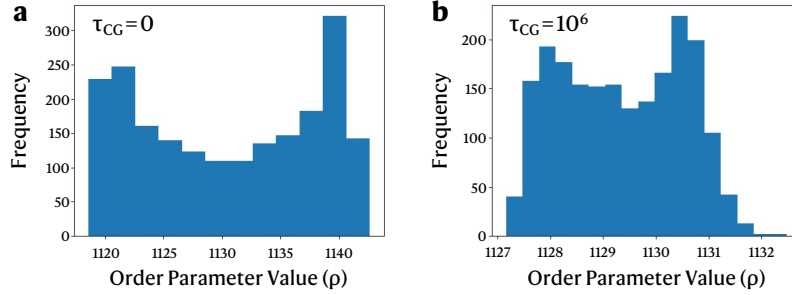

FIG. S3. Comparison of the microscopic order parameter  $\rho$  distributions between (a)  $\tau_{CG} = 0$  and (b)  $\tau_{CG} = 10^6$ . The clear bimodal distribution between water and ice is exhibited at  $\tau_{CG} = 0$ , highlighting the fidelity of  $\rho$  as an order parameter to distinguish ice nucleation.

From the histogram distribution, the average  $\langle a_I \rangle$  is approximately 554 ( $\text{\AA}^2$ ). To effectively account for the non-zero distance distribution, we set the variance  $c$  to be  $554 / \ln 2 \approx 800$  ( $\text{\AA}^2$ ). The time evolution of the designed  $\langle \rho_I \rangle$  shown in Fig. 1(a) confirms that this  $c$  parameter provides well-defined scale for the Gaussian form of  $\rho_I$ . Note that  $c$  will depend in general on thermodynamic state point variables.

## 2. Efficacy of $\rho_I$ at the water/ice interface

Using the local density  $\rho_I$  defined in Eq. (3) from Fig. S2, we proceed to design a microscopic phase-field variable  $\phi_I$  capable of distinguishing between ice and water phases. This activation function is typically represented using a sigmoidal function, employing the hyperbolic tangent function:

$$\phi_I = \frac{1}{2} \left( 1 - \tanh \left( \frac{\rho_I - \rho_0}{\Delta \rho} \right) \right). \quad (\text{S2})$$

To determine the optimal parameters  $\rho_0$  and  $\Delta \rho$  for  $\phi_I$  in Eq. (S2), we evaluated the histogram of the single CG MD configuration at the initial condition ( $\tau_{CG} = 0$ ) and the final condition ( $\tau_{CG} = 10^6$ ). Note that the  $\tau_{CG} = 0$  condition contains both water and ice phases, while  $\tau_{CG} = 10^6$  predominantly consists of the ice phase with lattice vibration dynamics. Figure S3 illustrates two distinct histograms, where the ice phase exhibits relatively lower  $\rho$  values compared to the higher  $\rho$  values in water, as expected. Notably, Fig. S2(a) demonstrates a clear bimodal distribution of water and ice phases separated near  $\rho \approx 1132$ , as the unimodal distribution decays after  $\rho > 1132$  in Fig. S2(b). Therefore, we selected  $\rho_0 = 1132$  and  $\Delta \rho = 2$  to cover the bimodal distribution, which is shown to effectively distinguish between water and ice phases in our simulations as depicted in Fig. 1(c) for  $\phi_I$ .

## B. Derivation of Microscopic Hamiltonian [Eq. (5)]

### 1. Coarse-Graining with Internal States: Theory of Ultra-Coarse-Graining

When deriving a microscopic Hamiltonian for the ice-water interface at the molecular CG level capable of distinguishing between solid and liquid phases [S1, S2], conventional CG methods fail to differentiate between phases as they treat molecular entities identically [S3–S5]. Therefore, a new methodology is required. Herein, we introduce the ultra-coarse-graining methodology [S6–S8], which defines internal states beneath CG sites to capture phase-specific information omitted by conventional CG models. We first outline the foundational assumptions and rationale behind the ultra-coarse-graining theory.

Consider a CG system in CG phase space  $(\mathbf{R}^N, \mathbf{P}^N)$  with an effective CG free energy  $U(\mathbf{R}^N)$ . Conventionally,  $U(\mathbf{R}^N)$  employs a pairwise approximation

$$U(\mathbf{R}^N) = \sum_{I,J} U(R_{IJ}). \quad (\text{S3})$$

Next, we introduce the internal states underlying each CG particle. In order to impose internal states that change their identity (e.g., between different phases), these states should be described by the particle’s chemical information [S6–S8]. It is reasonable to further assume that these internal states are determined by the CG particle’s *local* chemical environment. As the CG particle translates during the simulation, the internal states will rapidly adjust their identity based on the changed environment. Hence, there is a separation of time scales between the CG translational dynamics (slow) and internal state dynamics (rapid), similar to the Ehrenfest dynamics at the quantum level.

Under this “rapid local equilibrium” limit of internal states, the effective CG particle can be described as a linear combination of different internal states with quasi-equilibrium internal state probabilities. Thus, the CG Hamiltonian can be reformulated in terms of internal state variables  $\{s_I\}$  for CG site  $I$  [S8, S9]:

$$U(\mathbf{R}^N) = \sum_{I,J} \sum_{s_I, s_J} p_{I,s_I}(R_{IJ}|\mathbf{R}^N) p_{J,s_J}(R_{IJ}|\mathbf{R}^N) U_{s_I, s_J}(R_{IJ}), \quad (\text{S4})$$

where  $U_{s_I, s_J}(R_{IJ})$  denotes the statewise interaction under the pairwise approximation, and the internal state probability  $p_{I,s_I}(R_{IJ}|\mathbf{R}^N)$  is conditioned on the overall CG configuration  $\mathbf{R}^N$ , implying the locality of internal states and the time scale separation.

The critical steps for implementing Eq. (S4) involve (1) selecting an effective (microscopic) order parameter capable of distinguishing between different internal states  $\{s_I\}$ , and (2) designing an appropriate internal state probability function  $p_{I,s_I}(R_{IJ}|\mathbf{R}^N)$  that can capture the order parameter distribution from the reference system, and (3) determining the statewise interactions using bottom-up methodologies to correctly reflect the underlying free energies [S10].

### 2. Derivation of Eq. (5)

We now apply the internal state CG approach to our water-ice interface. In this interface system, the state variable can be categorized as  $\{(s), (l)\}$ , corresponding to solid-like and liquid-like states, respectively [S11]. The use of “-like state” acknowledges that these internal state descriptions may not be exactly identical to the “actual” phases observed at the atomistic level.

Also, unlike conventional approaches, we assume that our CG Hamiltonian is no longer strictly pairwise but dependent on an order parameter [S12]. Here, we choose this order parameter from the main text ( $\rho_I$ ) to design  $U_{\text{CG}}$

$$U_{\text{CG}} = U(\{\rho_I\}_I, \mathbf{R}^N) = \sum_I U_I(\rho_I), \quad (\text{S5})$$

where  $U_I(\rho_I)$  can be understood as an effective chemical potential that depends on the local environment of the CG particle  $I$  given by  $\rho_I = \sum_{J \neq I} \left[ \exp \left( -\frac{(\mathbf{R}_I - \mathbf{R}_J)^2}{800} \right) \right]$ . Thus, despite its one-body form,  $U_I(\rho_I)$  encodes the many-body nature into the CG free energy, as  $U_I$  contains  $\rho_I$  that depends on the local environment. Meanwhile,  $\phi_I$  retains an effective pairwise nature, and choosing a  $\phi_I$  basis will not change any of our previous arguments using the spatial  $\{R_{IJ}\}$  basis.

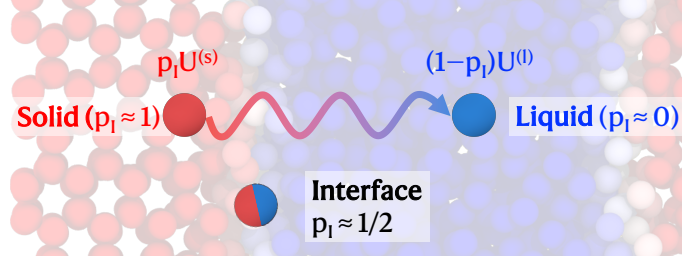

FIG. S4. Internal-state CG approach (ultra-coarse-graining) for describing CG representation of solid-liquid interface. The effective bulk CG Hamiltonian is described as a linear combination of the solid-like contribution  $p_I U^{(s)}$  and the liquid-like contribution  $(1 - p_I) U^{(l)}$ , where  $p_I$  is the solid-like probability defined by the microscopic order parameter  $\rho$  and  $\rho_I = 1/2$  at the interface. Combined with the interfacial contribution, Eq. (S11) serves as the molecular-level representation of the phase-field Hamiltonian.

We proceed by introducing the internal state approach to Eq. (S5) to differentiate between solid and liquid phases. Under quasi-equilibrium conditions, the internal state approach of the one-body Hamiltonian yields

$$U(\mathbf{R}^N) = \sum_I p_{I,s_I}(\rho_I | \mathbf{R}^N) U_{s_I}(\rho_I) = \sum_I \left( p_I U^{(s)}(\rho_I) + (1 - p_I) U^{(l)}(\rho_I) \right), \quad (\text{S6})$$

where  $p_I := p_{I,s_I}(\rho_I | \mathbf{R}^N)$  denotes the solid-like internal state probability ( $s_I$ ). Since the quasi-equilibrium condition in Eq. (S6) is a direct consequence of the time scale separation between the internal state dynamics and CG particle translation, it does not require any additional conditions. Hence, we note that, in principle, Eq. (S6) can be utilized to describe both equilibrium (Boltzmann weighted) and non-equilibrium growth processes.

Nevertheless, Eq. (S6) may not fully capture the heterogeneous nature of the interface due to the excess free energy  $U_{\text{interface}}(\rho_I)$  from interfacial fluctuations. Therefore, one can express the free energy of the interface as

$$U(\phi, \mathbf{R}^N) = \sum_I (p_I U^{(s)}(\rho_I) + (1 - p_I) U^{(l)}(\rho_I)) + \sum_I U_{\text{interface}}(\rho_I), \quad (\text{S7})$$

where we introduce the bulk chemical potentials  $U^{(s)}(\rho_I)$  and  $U^{(l)}(\rho_I)$  as functions of the microscopic density, independent of particle index. The overall free energy is then expressed as an effective average using the conditional solid probability  $p_I = p_I(\rho_I | \mathbf{R}^N)$  conditioned to the CG configurations. The additional free energy term for the interface,  $U_{\text{interface}}(\rho_I)$ , can be further described as fluctuations in the interface height  $h(\mathbf{R}^N)$ , defined as the distance from the center of the system (e.g., Willard-Chandler interface [S13]) using the capillary wave theory (CWT) [S14, S15]. With the CWT under the small gradient approximation, the excess interface Hamiltonian can be represented as

$$\sum_I U_{\text{interface}}(\rho_I) = \int d\mathbf{R}^N \{ g(h(\mathbf{R}^N)) + \gamma |\nabla h(\mathbf{R}^N)|^2 \}, \quad (\text{S8})$$

where the local free energy  $g(h(\mathbf{R}^N))$  is an unshifted interface free energy containing terms that are independent of the gradient of  $h(\mathbf{R}^N)$  [S15]. As  $g(h(\mathbf{R}^N))$  is still dependent on the interface height, we introduce a new conditional probability  $q_I = q_I(\rho_I | \mathbf{R}^N)$  of being at the interface to capture this dependency. Then, the first term on the right-hand side of Eq. (S8) can be rewritten as

$$\int d\mathbf{R}^N g(h(\mathbf{R}^N)) = \sum_I q_I \Delta U(\rho_I), \quad (\text{S9})$$

where  $\Delta U(\rho_I)$  denotes the excess free energy that corresponds to the limit of an infinitely thick interface. Next, the remaining gradient term with a surface tension-like coefficient  $\gamma$  can alternatively be expressed as [S14, S16]

$$\int d\mathbf{R}^N \gamma |\nabla h(\mathbf{R}^N)|^2 \approx \sum_I \frac{\epsilon^2}{2} |\nabla \rho_I|^2. \quad (\text{S10})$$

Combining these contributions yields the finalized microscopic expression for the CG free energy:

$$U(\mathbf{R}^N) = \sum_I (p_I U^{(s)}(\rho_I) + (1 - p_I) U^{(l)}(\rho_I)) + \sum_I q_I \Delta U(\rho_I) + \sum_I \frac{\epsilon^2}{2} |\nabla \rho_I|^2, \quad (\text{S11})$$

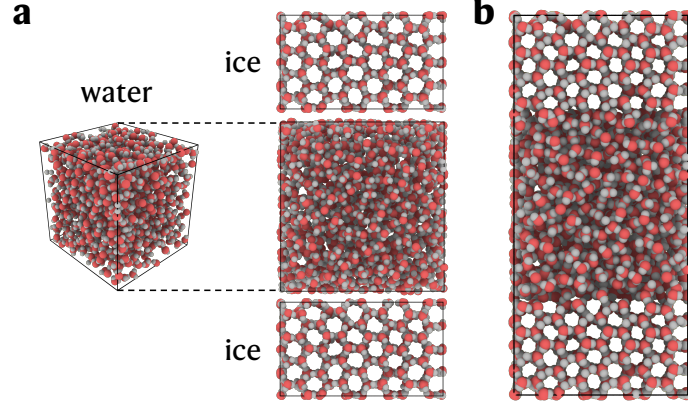

FIG. S5. Construction of the ice-water interface at the atomistic level. (a) From the equilibrated structure of the liquid water, ice slabs following the algorithm by Buch et al. [S17] are inserted to construct the solid-liquid interface. (b) After energy minimization to remove artificial stress, the equilibrated interface snapshot during the atomistic MD simulation is shown.

which can be effectively considered as  $U(\mathbf{R}^N) = \sum_I (U_{\text{bulk}}(\rho_I) + U_{\text{interface}}(\rho_I))$ , where  $U_{\text{bulk}}(\rho_I) = (p_I U^{(s)}(\rho_I) + (1 - p_I) U^{(l)}(\rho_I))$ . The additive coupling between  $U_{\text{bulk}}$  and  $U_{\text{interface}}$  implies a separation of time scales between interface fluctuations and the particle reorientation, underscoring our model's ability to capture long-wavelength fluctuations from the interface while incorporating one-body terms that effectively describe the bulk free energy along the CG free energy surfaces.

As Eq. (S11) can faithfully represent the microscopic representation of the phase-field free energy, we now consider an additional order parameter mapping (one-to-one) from  $\rho_I$  to the microscopic phase-field variable  $\phi_I$  as given in Eq. (4). Finally, switching the variables from  $\rho_I$  to  $\phi_I$  gives

$$U(\phi, \mathbf{R}^N) = \sum_I \left( p(\phi_I) f_s(\phi_I) + (1 - p(\phi_I)) f_l(\phi_I) + W(\phi_I) q(\phi_I) + f_\epsilon(\phi_I) |\nabla_I \phi_I|^2 \right),$$

which corresponds to  $\mathcal{F}^{\text{CG}}$  in Eq. (5) by defining the microscopic free energy densities as  $W(\phi_I) := \Delta U_I$  and  $f_\epsilon(\phi_I) := \epsilon^2/2$ . ■

### III. ATOMISTIC LEVEL

#### A. Atomistic Simulation Setup

Building upon previous studies of the ice-water interface in the literature, we construct an atomistic ice-water interface model to investigate the detailed mechanisms underlying crystal growth. Following recent CG studies on the ice-water interface [S1, S2], we constructed the CG interface ( $N = 2048$ ) composed of  $N_l = 1024$  water and  $N_s = 1024$  ice molecules. The initial water structure was centered within the simulation box, and the size of the simulation box was determined by the experimental density. The liquid box was capped with 512 ice molecules on both top and bottom, respectively. The initial structure of water liquid was randomized, whereas the ice configuration was initialized with zero dipole moments using the algorithm from Ref. S17, see Fig. S5(a). After constant NVT runs of each component, we constructed the slab configurations by merging the three components together. The final simulation box dimensions were  $31.50 \times 29.84 \times 68.58$  ( $\text{\AA}^3$ ), as illustrated in Fig. S5(b). The atomistic simulation followed the protocol described in Ref. [S2] using the TIP4P/Ice force field [S18] at the undercooled condition  $T = 249$  K and  $P = 1$  atm.

#### B. Three-body CG Model for Water

In order to expedite ice growth at the interface, we constructed a molecular CG model based on the atomistic simulation trajectory. In particular, since three-body correlations in water are crucial for describing hydrogen bonding

and ice structure [S19], we adopted effective three-body interactions to model the CG Hamiltonian  $U(\mathbf{R}^N)$  [S20]:

$$U(\mathbf{R}^N) = \sum_I \sum_{J \neq I} U^{(2)}(R_{IJ}) + \sum_I \sum_{J \neq I} \sum_{K > J} U^{(3)}(\theta_{JIK}, R_{IJ}, R_{IK}), \quad (\text{S12})$$

where  $U^{(2)}$  and  $U^{(3)}$  denote two-body and three-body interactions, respectively. In particular, inspired by the monatomic water (mW) model [S21], the Stillinger-Weber potential [S22] was utilized for  $U^{(3)}$ :

$$U^{(3)}(\theta_{JIK}, R_{IJ}, R_{IK}) = \lambda_{JIK} (\cos \theta_{jik} - \cos \theta_0)^2 \exp\left(\frac{\gamma_{IJ}}{R_{IJ} - a_{IJ}}\right) \exp\left(\frac{\gamma_{IK}}{R_{IK} - a_{IK}}\right) \quad (\text{S13})$$

where  $\gamma_{JIK}$  determines the interaction strength, and  $a_{IJ}$  and  $a_{IK}$  are the cutoff distances. For water, we closely followed the original parametrization protocol [S3]:  $\gamma_{IJ} = 1.2$ ,  $\sigma_{IJ} = 1$  Å,  $\epsilon_{JIK} = 1.0$  kcal/mol, with a cutoff  $a_{IJ} = 3.7$  Å. Then, the bottom-up determination of  $U^{(2)}$  and  $\lambda_{JIK}$  for  $U^{(3)}$  was achieved by variational force-matching [S3], yielding  $\lambda_{JIK} = 28.0078$  at 249 K. Detailed parametrization procedure and discussion can also be found in [S1, S2].

### C. CG Simulation Details

From the last snapshot of the atomistic MD simulation, water molecules were manually mapped to their center-of-masses and used as the initial configuration for the CG simulation ( $\tau_{\text{CG}} = 0$ ). We then performed a constant  $NVT$  simulation for 10 ns ( $\tau_{\text{CG}} = 2 \times 10^6$ ) using a Nosé-Hoover thermostat with a coupling constant of 100 fs [S23, S24].

## IV. VARIATIONAL COARSE-GRAINING

### A. Molecular Coarse-Graining

Here, we elaborate on how to determine the microscopic free energy density  $f_s(\phi_I)$ ,  $f_l(\phi_I)$ ,  $f_w(\phi_I)$ , and  $f_\epsilon(\phi_I)$  variationally. Without loss of generality, we start with  $f_s(\phi_I)$ . From the spline representation,  $f_s(\phi_I) = \sum_k c_k^s B_k^s(\phi_I)$ , where the spline coefficient  $\{c_k^s\}_k$  can be determined via the corresponding force  $\mathbf{F}_I^s$  by variational optimization:

$$\begin{aligned} \mathbf{F}_I^s &= -\nabla_I \left( \sum_J \bar{p}(\phi_J) f_s(\phi_J) \right) \\ &= -\sum_J \left( \bar{p}(\phi_J) \frac{\partial f_s(\phi_J)}{\partial \phi_J} \frac{\partial \phi_J}{\partial \mathbf{R}_I} + f_s(\phi_J) \frac{\partial \bar{p}(\phi_J)}{\partial \phi_J} \frac{\partial \phi_J}{\partial \mathbf{R}_I} \right) \\ &= -\sum_J \sum_k \left( \left[ c_k^s \bar{p}(\phi_J) \frac{\partial \phi_J}{\partial \mathbf{R}_I} \right] B_k^{s'}(\phi_J) + \left[ c_k^s f_s(\phi_J) \frac{\partial \bar{p}(\phi_J)}{\partial \phi_J} \frac{\partial \phi_J}{\partial \mathbf{R}_I} \right] B_k^s(\phi_J) \right), \end{aligned} \quad (\text{S14})$$

which simplifies to

$$\mathbf{F}_I^s = -\sum_{J,k} \left( c_k^s \left[ \bar{p}(\phi_J) \frac{\partial \phi_J}{\partial \mathbf{R}_I} B_k^{s'}(\phi_J) + \dot{\bar{p}}(\phi_J) \frac{\partial \phi_J}{\partial \mathbf{R}_I} B_k^s(\phi_J) \right] \right). \quad (\text{S15})$$

In turn, the first step of molecular coarse-graining introduces the phenomenological  $\bar{p}(\phi_I)$  to Eq. (S15) for linearizing  $\mathbf{F}_I^s$ , and hence

$$\mathbf{F}_I^s = -\sum_{J,k} \left( c_k^s \left[ (\phi_J^3(10 - 15\phi_J + 6\phi_J^2)) \frac{\partial \phi_J}{\partial \mathbf{R}_I} B_k^{s'}(\phi_J) + (30(1 - \phi_J)^2 \phi_J^2) \frac{\partial \phi_J}{\partial \mathbf{R}_I} B_k^s(\phi_J) \right] \right). \quad (\text{S16})$$

Now, Eq. (S16) is linear in terms of  $c_k^s$ , and force-matching [Eq. (6) in the main text] can variationally determine  $\{c_k^s\}_k$ .

Similarly, the liquid free energy density,  $f_l(\phi_I) = \sum_k c_k^l B_k^l(\phi_I)$ , is directly related to  $f_s$  via  $(1 - \bar{p}(\phi_I))$ , giving

$$\mathbf{F}_I^l = -\sum_{J,k} \left( c_k^l \left[ \{(1 - \phi_J)^3(1 + 3\phi_J + 6\phi_J^2)\} \frac{\partial \phi_J}{\partial \mathbf{R}_I} B_k^{l'}(\phi_J) - (30(1 - \phi_J)^2 \phi_J^2) \frac{\partial \phi_J}{\partial \mathbf{R}_I} B_k^l(\phi_J) \right] \right). \quad (\text{S17})$$

Next, the effective force exerted by the double-well free energy  $f_w(\phi_I) = \sum_k c_k^w B_k^w(\phi_I)$  can also be expressed using the phenomenological  $\bar{q}(\phi_J) = \phi_J^2(1 - \phi_J)^2$  and its derivative  $\bar{q}'(\phi_J) = 2\phi_J(\phi_J - 1)(2\phi_J - 1)$ , resulting in

$$\mathbf{F}_I^w = - \sum_{J,k} \left( c_k^w \left[ \{ \phi_J^2(1 - \phi_J)^2 \} \frac{\partial \phi_J}{\partial \mathbf{R}_I} B_k^{w'}(\phi_J) + 2\phi_J(\phi_J - 1)(2\phi_J - 1) \frac{\partial \phi_J}{\partial \mathbf{R}_I} B_k^w(\phi_J) \right] \right). \quad (\text{S18})$$

Finally, we express the gradient free energy  $f_\epsilon$  contributing to the overall free energy as

$$\mathcal{F}_{grad} = \sum_J (\nabla_J \phi_J)^2 f_\epsilon(\phi_J), \quad (\text{S19})$$

where we have absorbed  $\epsilon^2(\phi_J)$  into  $f_\epsilon(\phi_J)$  for notational convenience. Now, the effective force expressed by  $\mathcal{F}_{grad}$  is

$$\mathbf{F}_I^\epsilon = -\nabla_I \mathcal{F}_{grad} = - \sum_J \left[ (\nabla_J \phi_J)^2 \frac{\partial f_\epsilon(\phi_J)}{\partial \phi_J} \frac{\partial \phi_J}{\partial \mathbf{R}_I} + 2f_\epsilon(\phi_J) (\nabla_J \phi_J) \nabla_I (\nabla_J \phi_J) \right]. \quad (\text{S20})$$

Introducing the spline representation  $f_\epsilon(\phi_I) = \sum_k c_k^\epsilon B_k^\epsilon(\phi_I)$  further simplifies Eq. (S20) to

$$\mathbf{F}_I^\epsilon = - \sum_{J,k} \left( c_k^\epsilon \left[ (\nabla_J \phi_J)^2 B_k^{\epsilon'}(\phi_J) \frac{\partial \phi_J}{\partial \mathbf{R}_I} + 2B_k^\epsilon(\phi_J) (\nabla_J \phi_J) \nabla_I (\nabla_J \phi_J) \right] \right). \quad (\text{S21})$$

Note that by design Eq. (S21) does not contain any *ad hoc* polynomials, and coefficients  $(\nabla_J \phi_J)^2$  and  $(\nabla_J \phi_J) \nabla_I (\nabla_J \phi_J)$  can be readily sampled from microscopic trajectories. We would like to note that the key takeaway of Eqs. (S20) and (S21) is that  $\mathbf{F}_I^\epsilon$  is linear in terms of the spline coefficients  $\{c_k^\epsilon\}_k$  like  $\mathbf{F}_I^s$ ,  $\mathbf{F}_I^l$ , and  $\mathbf{F}_I^w$ . The analytical form for these coefficients will be given in the next subsection.

Combined these, the total force  $\mathbf{F}_I$  is expressed as

$$\mathbf{F}_I = \mathbf{F}_I^s + \mathbf{F}_I^l + \mathbf{F}_I^w + \mathbf{F}_I^\epsilon, \quad (\text{S22})$$

as all free energy components are linear. Thus, force matching on the total force ( $\mathbf{F}_I$ ) level becomes a set of linear equations:

$$\begin{aligned} \mathbf{F}_I = - \sum_{J,k} \left( \left\{ c_k^s \left[ (\phi_J^3(10 - 15\phi_J + 6\phi_J^2)) \frac{\partial \phi_J}{\partial \mathbf{R}_I} B_k^{s'}(\phi_J) + (30(1 - \phi_J)^2 \phi_J^2) \frac{\partial \phi_J}{\partial \mathbf{R}_I} B_k^s(\phi_J) \right] \right\} \right. \\ + \left\{ c_k^l \left[ \{(1 - \phi_J)^3(1 + 3\phi_J + 6\phi_J^2)\} \frac{\partial \phi_J}{\partial \mathbf{R}_I} B_k^{l'}(\phi_J) - (30(1 - \phi_J)^2 \phi_J^2) \frac{\partial \phi_J}{\partial \mathbf{R}_I} B_k^l(\phi_J) \right] \right\} \\ + \left\{ c_k^w \left[ \{\phi_J^2(1 - \phi_J)^2\} \frac{\partial \phi_J}{\partial \mathbf{R}_I} B_k^{w'}(\phi_J) + 2\phi_J(\phi_J - 1)(2\phi_J - 1) \frac{\partial \phi_J}{\partial \mathbf{R}_I} B_k^w(\phi_J) \right] \right\} \\ \left. + \left\{ c_k^\epsilon \left[ (\nabla_J \phi_J)^2 B_k^{\epsilon'}(\phi_J) \frac{\partial \phi_J}{\partial \mathbf{R}_I} + 2B_k^\epsilon(\phi_J) (\nabla_J \phi_J) \nabla_I (\nabla_J \phi_J) \right] \right\} \right), \quad (\text{S23}) \end{aligned}$$

and the variational force-matching [Eq. (6)] can determine the spline coefficients in Eq. (S23).

## B. Analytical Form

### 1. Bulk free energy

To evaluate Eqs. (S16)–(S18) analytically, we need to determine  $\partial \phi_J / \partial \mathbf{R}_I$  from our definition of  $\phi_J$  [Eq. (3)]. Despite its complexity, we can simplify the analysis by considering two cases: when  $J \neq I$  or otherwise  $J = I$ . For simplicity, we omit the units for now, but they adhere to the definitions in Eqs. (3) and (4). Specifically, for the case when  $J = I$ , we have

$$\begin{aligned} \frac{\partial \phi_I}{\partial \mathbf{R}_I} &= -\frac{1}{2} \text{sech}^2 \left[ \frac{\rho_I - 1132}{2} \right] \frac{1}{2} \frac{\partial \rho_I}{\partial \mathbf{R}_I} \\ &= -\frac{1}{4} \text{sech}^2 \left[ \frac{\rho_I - 1132}{2} \right] \sum_{K \neq I} \left[ \exp \left( -\frac{(\mathbf{R}_I - \mathbf{R}_K)^2}{800} \right) \cdot \left( -\frac{2(\mathbf{R}_I - \mathbf{R}_K)}{800} \right) \right], \quad (\text{S24}) \end{aligned}$$

because  $\partial\rho_I/\partial\mathbf{R}_I$  is defined as

$$\frac{\partial\rho_I}{\partial\mathbf{R}_I} = \sum_{K \neq I} \left[ \exp\left(-\frac{(\mathbf{R}_I - \mathbf{R}_K)^2}{800}\right) \cdot \left(-\frac{2(\mathbf{R}_I - \mathbf{R}_K)}{800}\right) \right]. \quad (\text{S25})$$

Similarly,  $\partial\phi_J/\partial\mathbf{R}_I$  for  $J \neq I$  is

$$\begin{aligned} \frac{\partial\phi_J}{\partial\mathbf{R}_I}|_{J \neq I} &= -\frac{1}{4}\text{sech}^2\left[\frac{\rho_J - 1132}{2}\right] \frac{\partial\rho_J}{\partial\mathbf{R}_I} \\ &= -\frac{1}{4}\text{sech}^2\left[\frac{\rho_J - 1132}{2}\right] \cdot \left[ \exp\left(-\frac{(\mathbf{R}_J - \mathbf{R}_I)^2}{800}\right) \cdot \frac{2(\mathbf{R}_J - \mathbf{R}_I)}{800} \right]. \end{aligned} \quad (\text{S26})$$

Equations (S24) and (S25) are crucial for deriving the analytical expression of  $\mathbf{F}_I$ .

## 2. Gradient free energy

Now, we turn to deriving an analytical form of the coefficients in Eqs. (S20) and (S21) for the force-matching procedure. In Eq. (S20), the first term resembles the other free energy forces, whereas the complexity arises from the cross-nabla term  $(\nabla_J\phi_J)\nabla_I(\nabla_J\phi_J)$ . Therefore, for simplicity, we will only outline how the second term can be further evaluated. Similar to the evaluation of  $\partial\phi_J/\partial\mathbf{R}_I$ , we decompose this into contributions from  $J \neq I$  and  $J = I$  in the summation, i.e.,

$$-\sum_J [2\epsilon(\phi_J)(\nabla_J\phi_J)\nabla_I(\nabla_J\phi_J)] = -2\epsilon \left[ (\nabla_I\phi_I)\nabla_I^2\phi_I + \sum_{J \neq I} (\nabla_J\phi_J)\nabla_I(\nabla_J\phi_J) \right]. \quad (\text{S27})$$

For clarity, we again define the prefactor  $f(\phi_J)$  as

$$f(\phi_J) := -\frac{1}{4}\text{sech}^2\left(\frac{\rho_J - 1132}{2}\right). \quad (\text{S28})$$

and rewrite  $\nabla_J\phi_J$  as

$$\begin{aligned} \nabla_J\phi_J &= -\frac{1}{4}\text{sech}^2\left(\frac{\rho_J - 1132}{2}\right) \sum_{K \neq J} \left[ \exp\left(-\frac{(\mathbf{R}_J - \mathbf{R}_K)^2}{800}\right) \cdot \left(-\frac{2(\mathbf{R}_J - \mathbf{R}_K)}{800}\right) \right] \\ &= f(\rho_J) \frac{\partial\rho_J}{\partial\mathbf{R}_J}, \end{aligned} \quad (\text{S29})$$

where  $\partial\rho_J/\partial\mathbf{R}_J = \sum_{K \neq J} \left( \exp\left(-\frac{(\mathbf{R}_J - \mathbf{R}_K)^2}{800}\right) \cdot \left(-\frac{2(\mathbf{R}_J - \mathbf{R}_K)}{800}\right) \right)$ . This allows us to simplify the second term contribution from  $J \neq I$ :

$$\begin{aligned} \mathbf{F}_I^{(2)} &= -2\epsilon \sum_{J \neq I} \left[ f(\rho_J) \left\{ \sum_{K \neq J} \left( \exp\left(-\frac{(\mathbf{R}_J - \mathbf{R}_K)^2}{800}\right) \cdot \left(-\frac{2(\mathbf{R}_J - \mathbf{R}_K)}{800}\right) \right) \right\} \times \left\{ \frac{\partial f(\rho_J)}{\partial\rho_J} \cdot \exp\left(-\frac{(\mathbf{R}_J - \mathbf{R}_I)^2}{800}\right) \right. \right. \\ &\quad \cdot \left. \left. \left( \frac{2(\mathbf{R}_J - \mathbf{R}_I)}{800} \right) \cdot \left\{ \sum_{K \neq J} \left( \exp\left(-\frac{(\mathbf{R}_J - \mathbf{R}_K)^2}{800}\right) \cdot \left(-\frac{2(\mathbf{R}_J - \mathbf{R}_K)}{800}\right) \right) \right\} \right\} + f(\rho_J) \exp\left(-\frac{(\mathbf{R}_J - \mathbf{R}_I)^2}{800}\right) \right. \\ &\quad \cdot \left. \left\{ \left( \frac{2(\mathbf{R}_J - \mathbf{R}_I)}{800} \right)^2 + \frac{2}{800} \right\} \right], \end{aligned} \quad (\text{S30})$$

which can be further simplified using the definition of  $\partial\rho_J/\partial\mathbf{R}_J$

$$\begin{aligned} \mathbf{F}_I^{(2)} &= -2\epsilon \sum_{J \neq I} \left[ \left\{ f(\rho_J) \frac{\partial\rho_J}{\partial\mathbf{R}_J} \cdot \left( \frac{\partial f(\rho_J)}{\partial\rho_J} \exp\left(-\frac{(\mathbf{R}_J - \mathbf{R}_I)^2}{800}\right) \cdot \left( \frac{2(\mathbf{R}_J - \mathbf{R}_I)}{800} \right) \cdot \frac{\partial\rho_J}{\partial\mathbf{R}_J} \right\} \right. \\ &\quad \left. + f(\rho_J) \cdot \exp\left(-\frac{(\mathbf{R}_J - \mathbf{R}_I)^2}{800}\right) \left\{ \left( \frac{2(\mathbf{R}_J - \mathbf{R}_I)}{800} \right)^2 + \frac{2}{800} \right\} \right]. \end{aligned} \quad (\text{S31})$$

For  $J = I$ , the contribution simplifies to

$$\begin{aligned} \mathbf{F}_I^{(1)} = & -2\epsilon f(\rho_I) \sum_{K \neq I} \left[ \exp\left(-\frac{(\mathbf{R}_I - \mathbf{R}_K)^2}{800}\right) \cdot \left(-\frac{2(\mathbf{R}_I - \mathbf{R}_K)}{800}\right) \right] \times \left[ \frac{\partial f(\rho_I)}{\partial \rho_I} \right. \\ & \cdot \left( \sum_{K \neq I} \left[ \exp\left(-\frac{(\mathbf{R}_I - \mathbf{R}_K)^2}{800}\right) \cdot \left(-\frac{2(\mathbf{R}_I - \mathbf{R}_K)}{800}\right) \right] \right)^2 + f(\rho_I) \times \left( \sum_{K \neq I} \exp\left(-\frac{(\mathbf{R}_I - \mathbf{R}_K)^2}{800}\right) \right. \\ & \left. \left. \times \left\{ \left( \frac{2(\mathbf{R}_I - \mathbf{R}_K)}{800} \right)^2 - \frac{2}{800} \right\} \right) \right]. \end{aligned} \quad (\text{S32})$$

Note that here we have used

$$\frac{\partial \rho_I}{\partial \mathbf{R}_I} = \sum_{K \neq I} \left[ \exp\left(-\frac{(\mathbf{R}_I - \mathbf{R}_K)^2}{800}\right) \cdot \left(-\frac{2(\mathbf{R}_I - \mathbf{R}_K)}{800}\right) \right], \quad (\text{S33})$$

to further simplify  $\mathbf{F}_I^{(1)}$ , resulting in

$$\mathbf{F}_I^{(1)} = -2\epsilon f(\rho_I) \frac{\partial \rho_I}{\partial \mathbf{R}_I} \times \left[ \frac{\partial f(\rho_I)}{\partial \rho_I} \left( \frac{\partial \rho_I}{\partial \mathbf{R}_I} \right)^2 + f(\rho_I) \times \left( \sum_{K \neq I} \exp\left(-\frac{(\mathbf{R}_I - \mathbf{R}_K)^2}{800}\right) \times \left\{ \left( \frac{2(\mathbf{R}_I - \mathbf{R}_K)}{800} \right)^2 - \frac{2}{800} \right\} \right) \right]. \quad (\text{S34})$$

Due to the specific form of  $f(\rho_J)$ , its derivative with respect to  $\rho_J$  is given by

$$\frac{\partial f(\rho_J)}{\partial \rho_J} = \frac{1}{4} \tanh\left(\frac{\rho_J - 1132}{2}\right) \text{sech}^2\left(\frac{\rho_J - 1132}{2}\right). \quad (\text{S35})$$

Altogether, Eqs. (S28), (S31), (S34), and (S35) provide the analytical expression for evaluating the gradient free energy force.

### C. Parametrization Details

From the CG trajectory of water at the center-of-mass resolution, we introduce fourth-order B-splines using a resolution of 0.04. Over the range of  $\phi = 0$  to 1, we reconstruct the free energy quantities every 0.02 value in  $\phi$ .

## V. PHASE-FIELD LEVEL

### A. System Setup

#### 1. Initial Condition

We construct a two-dimensional mesoscopic-level system with grids of  $n_x = 130$  and  $n_y = 60$ . The spacing of numerical grids imposes mesoscopic length scales of  $\Delta x = 0.5 \mu\text{m}$ , resulting in an interface size of  $30 \mu\text{m} \times 65 \mu\text{m}$ . The initial condition  $\phi_0$  follows Eq. (8) of the main text, where the solution of the equilibrium profile is superposed at the center of the interface. The two-dimensional profile of the initial structure is illustrated in Fig. S6.

#### 2. Mesoscopic interface free energy from microscopic free energies

For the phase-field representation of the free energy function [Eq. (1) in the main text],

$$\mathcal{F} = \int_V dV \left( p(\phi) f_s + (1 - (\phi)) f_l + f_w q(\phi) + \frac{\epsilon^2}{2} |\nabla \phi|^2 \right) \quad (\text{S36})$$

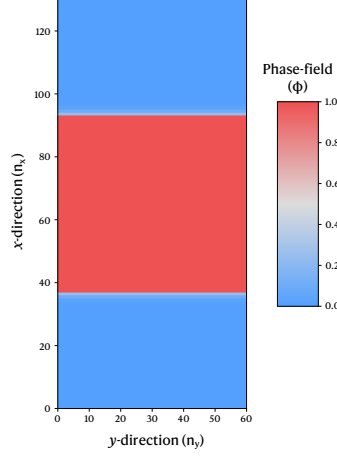

FIG. S6. Initial configuration of the microscopic phase-field model discretized on the numerical grid with  $n_x = 130$  and  $n_y = 60$ . The initial distribution  $\phi_0$  [Eq. (8) in the main text] is illustrated from  $\phi = 0$  (blue; water) to  $\phi = 1$  (red; ice).

the coefficients  $\epsilon$  and  $f_w$  are related to physical properties based on the relationships developed by Allen and Cahn [S25]. In particular, under the steady-state interface growth in one dimension, as derived in Ref. S26, we closely follow Ref. S27 to determine  $\epsilon$  and  $f_w$  [S28]

$$\epsilon = \sqrt{\frac{3\delta\gamma}{b}}, \quad (\text{S37})$$

$$f_w = \frac{6\gamma b}{\delta}, \quad (\text{S38})$$

where  $\delta$ ,  $\gamma$ , and  $b$  are defined in the main text. Given our definition of  $f_\epsilon := \epsilon^2/2$ , Eq. (S37) simplifies to

$$f_\epsilon = \frac{\epsilon^2}{2} = \frac{3\delta\gamma}{2b}, \quad (\text{S39})$$

as mentioned in the main text. Additionally, since we already have an mesoscopic value of  $f_w$ , expressing Eq. (S38) in terms of the interface width  $\gamma$  gives

$$\gamma = \frac{f_w \delta}{6b}. \quad (\text{S40})$$

Finally, we apply these relationships to our mesoscopic interface free energy density  $\mathfrak{e}$  to obtain  $\mathbb{f}_\epsilon$ .

### 3. Kinetic Coefficients

The dynamics of the phase-field variable are governed by the rescaled (phase-field) mobility  $M_\phi$ , which is related to the physical mobility of the interface between two phases,  $M$ , via [S28, S29]

$$M_\phi = \frac{\sqrt{2W}}{6a} M = 3.662 \times 10^5 M. \quad (\text{S41})$$

Given the conventional interfacial mobility of  $M = 10^{-6} \text{m}^4 \cdot \text{J}^{-1} \text{s}^{-1}$ , we arrive at  $M_\phi = 0.3662 \text{m}^3 \cdot \text{J}^{-1} \text{s}^{-1}$ , as stated in the main text.

## B. Phase-Field Simulation Details

We numerically discretized the Allen–Cahn equation using a finite difference method. First, we computed the functional derivative of  $\delta\mathcal{F}_{PF}/\delta\phi$ :

$$\begin{aligned}\frac{\delta\mathcal{F}_{PF}}{\delta\phi} &= \frac{\partial f_{chem}}{\partial\phi} + \frac{\partial f_{doub}}{\partial\phi} - \nabla \cdot \frac{\partial f_{grad}}{\partial(\nabla\phi)} \\ &= (\mathbb{f}_s - \mathbb{f}_l)p'_f(\phi) + \mathbb{f}_w q'_f(\phi) - 2\mathbb{f}_\epsilon \nabla^2\phi.\end{aligned}\quad (\text{S42})$$

We employed the first-order Euler method for time integration of  $\phi$ , and spatial derivatives were estimated using a second-order central finite difference scheme. In combination, the overall finite difference scheme is represented as

$$\begin{aligned}\phi(t + \Delta t)_{i,j} &= \phi(t)_{i,j} + M_\phi \left[ (\mathbb{f}_l - \mathbb{f}_s)p'_f(\phi) - \mathbb{f}_w q'_f(\phi) + 2\mathbb{f}_\epsilon^2 \left( \frac{\phi(t)_{i+1,j} - 2\phi(t)_{i,j} + \phi(t)_{i-1,j}}{(\Delta x)^2} \right. \right. \\ &\quad \left. \left. + \frac{\phi(t)_{i,j+1} - 2\phi(t)_{i,j} + \phi(t)_{i,j-1}}{(\Delta y)^2} \right) \right] \Delta t.\end{aligned}\quad (\text{S43})$$

To stably propagate  $\phi$ , we selected a small integration time step ( $\Delta t$ ) of

$$\Delta t = \frac{(\Delta x)^2}{10M_\phi\mathbb{f}_\epsilon^2} = 1.60 \times 10^{-7}(\text{s}), \quad (\text{S44})$$

which, by design, is within the microsecond range and consistent with the spatial scale of the system.

## VI. DATA AVAILABILITY

Jupyter Notebook for microscopic phase-field simulations and parametrization script in C++ programming language are available on GitHub [S30].

- 
- [S1] J. Jin, Y. Han, A. J. Pak, and G. A. Voth, A new one-site coarse-grained model for water: Bottom-up many-body projected water (bumper). i. general theory and model, *J. Chem. Phys.* **154**, 044104 (2021).
  - [S2] J. Jin, A. J. Pak, Y. Han, and G. A. Voth, A new one-site coarse-grained model for water: Bottom-up many-body projected water (bumper). ii. temperature transferability and structural properties at low temperature, *J. Chem. Phys.* **154**, 044105 (2021).
  - [S3] L. Larini, L. Lu, and G. A. Voth, The multiscale coarse-graining method. vi. implementation of three-body coarse-grained potentials, *J. Chem. Phys.* **132**, 164107 (2010).
  - [S4] L. Lu, J. F. Dama, and G. A. Voth, Fitting coarse-grained distribution functions through an iterative force-matching method, *J. Chem. Phys.* **139**, 121906 (2013).
  - [S5] C. Scherer and D. Andrienko, Understanding three-body contributions to coarse-grained force fields, *Phys. Chem. Chem. Phys.* **20**, 22387 (2018).
  - [S6] J. F. Dama, A. V. Sinitskiy, M. McCullagh, J. Weare, B. Roux, A. R. Dinner, and G. A. Voth, The theory of ultra-coarse-graining. 1. general principles, *Journal of chemical theory and computation* **9**, 2466 (2013).
  - [S7] A. Davtyan, J. F. Dama, A. V. Sinitskiy, and G. A. Voth, The theory of ultra-coarse-graining. 2. numerical implementation, *Journal of chemical theory and computation* **10**, 5265 (2014).
  - [S8] J. F. Dama, J. Jin, and G. A. Voth, The theory of ultra-coarse-graining. 3. coarse-grained sites with rapid local equilibrium of internal states, *J. Chem. Theory Comput.* **13**, 1010 (2017).
  - [S9] J. F. Dama, J. Jin, and G. A. Voth, Correction to the theory of ultra-coarse-graining. 3. coarse-grained sites with rapid local equilibrium of internal states, *Journal of Chemical Theory and Computation* **14**, 2288 (2018).
  - [S10] J. Jin, A. J. Pak, A. E. Durumeric, T. D. Loose, and G. A. Voth, Bottom-up coarse-graining: Principles and perspectives, *J. Chem. Theory Comput.* **18**, 5759 (2022).
  - [S11] J. Jin and G. A. Voth, Ultra-coarse-grained models allow for an accurate and transferable treatment of interfacial systems, *J. Chem. Theory Comput.* **14**, 2180 (2018).
  - [S12] J. W. Wagner, T. Dannenhoffer-Lafage, J. Jin, and G. A. Voth, Extending the range and physical accuracy of coarse-grained models: Order parameter dependent interactions, *J. Chem. Phys.* **147**, 044113 (2017).
  - [S13] A. P. Willard and D. Chandler, Instantaneous liquid interfaces, *J. Phys. Chem. B* **114**, 1954 (2010).

- [S14] J. S. Rowlinson and B. Widom, *Molecular theory of capillarity* (Courier Corporation, 2013).
- [S15] L. G. MacDowell, Capillary wave theory of adsorbed liquid films and the structure of the liquid-vapor interface, *Physical Review E* **96**, 022801 (2017).
- [S16] J. J. Hoyt, M. Asta, and A. Karma, Method for computing the anisotropy of the solid-liquid interfacial free energy, *Phys. Rev. Lett.* **86**, 5530 (2001).
- [S17] V. Buch, P. Sandler, and J. Sadlej, Simulations of h<sub>2</sub>o solid, liquid, and clusters, with an emphasis on ferroelectric ordering transition in hexagonal ice (1998).
- [S18] C. Vega and J. Abascal, Relation between the melting temperature and the temperature of maximum density for the most common models of water, *J. Chem. Phys.* **123**, 144504 (2005).
- [S19] U. Góra, R. Podeszwa, W. Cencek, and K. Szalewicz, Interaction energies of large clusters from many-body expansion, *J. Chem. Phys.* **135**, 224102 (2011).
- [S20] D. Hankins, J. Moskowitz, and F. Stillinger, Water molecule interactions, *The Journal of Chemical Physics* **53**, 4544 (1970).
- [S21] V. Molinero and E. B. Moore, Water modeled as an intermediate element between carbon and silicon, *J. Phys. Chem. B* **113**, 4008 (2009).
- [S22] F. H. Stillinger and T. A. Weber, Computer simulation of local order in condensed phases of silicon, *Phys. Rev. B* **31**, 5262 (1985).
- [S23] S. Nosé, A unified formulation of the constant temperature molecular dynamics methods, *J. Chem. Phys.* **81**, 511 (1984).
- [S24] W. G. Hoover, Canonical dynamics: Equilibrium phase-space distributions, *Phys. Rev. A* **31**, 1695 (1985).
- [S25] S. M. Allen and J. W. Cahn, A microscopic theory for antiphase boundary motion and its application to antiphase domain coarsening, *Acta Metall.* **27**, 1085 (1979).
- [S26] J. A. Warren and W. J. Boettinger, Prediction of dendritic growth and microsegregation patterns in a binary alloy using the phase-field method, *Acta Metall. Mater.* **43**, 689 (1995).
- [S27] T. Takaki, T. Fukuoka, and Y. Tomita, Phase-field simulation during directional solidification of a binary alloy using adaptive finite element method, *J. Cryst. Growth* **283**, 263 (2005).
- [S28] T. Takaki, Phase-field modeling and simulations of dendrite growth, *ISIJ Int.* **54**, 437 (2014).
- [S29] A. A. Wheeler, B. T. Murray, and R. J. Schaefer, Computation of dendrites using a phase field model, *Physica D* **66**, 243 (1993).
- [S30] The source code can be found in <https://github.com/jaehyeokjin/Bottom-up-Phase-Field>.
